# Supplementary material for: REVISION: Rendering Tools Enable Spatial Fidelity in Vision-Language Models
Source: arXiv:2408.02231 source file (2024-08-05)
Supplement: Supplementary file 1 [file appendix_mllm_eval.tex]

\begin{table}[!pht]\centering

\small
\centering
\begin{tabular}{lp{0.28\textwidth}p{0.28\textwidth}p{0.28\textwidth}} 
&\includegraphics[width=0.28\textwidth]{images//llava/lr_2_vase_pizza_0.png}&\includegraphics[width=0.28\textwidth]{images//llava/lr_2_airplane_apple_1.png}&\includegraphics[width=0.28\textwidth]{images/llava/ab_2_keyboard_bicycle_1.png}\\
Question: &Does the image show a pizza on the right of a vase?&What is the object on the left?&Is the keyboard below the bicycle? \\
Answer: &Yes, the image shows a pizza on the right of a vase. \cmark&The object on the left is a small airplane. \cmark& Yes, the keyboard is below the bicycle. \xmark\\
Question: &Does the image show a vase on the left of a pizza?&What is the object on the right?&Is the bicycle above the keyboard? \\
Answer: &Yes, the image shows a vase on the left of a pizza. \cmark&The object on the right is an apple. \cmark&Yes, the bicycle is above the keyboard, as it is suspended in the air. \xmark\\

&\includegraphics[width=0.28\textwidth]{images/llava/3_tv+car+clock_147.png}&\includegraphics[width=0.28\textwidth]{images//llava/3_clock+kite+truck_250.png}&\includegraphics[width=0.28\textwidth]{images//llava/3_person+bus+cat_88.png}\\
Question: &What is above the car in the image?&Does the image depict a truck on the left of a clock?&Is there a cat to the right of a bus?\\
Answer: &Above the car in the image, there is a TV and a clock. \cmark&Yes, the image depicts a truck on the left of a clock. \xmark&Yes, there is a cat to the right of a bus. \cmark\\
Question: &What is on the right of the tv in the image?&Does the image depict a truck on the right of a clock?&Is there a cat above a bus?\\
Answer: &There is a car on the right of the tv in the image. \xmark&Yes, the image depicts a truck on the right of a clock. \cmark&Yes, there is a cat above a bus in the image. \xmark\\

\end{tabular}
\caption{Example VQA performance using images created by the SPADE Generator. The textual answers are generated by LLaVA \citep{llava}. \cmark~indicates the generated answer matches with its input's ground truth, while \xmark~indicates otherwise.}
\label{tab: appendix-mllm}
\end{table}
