# Supplementary material for: REVISION: Rendering Tools Enable Spatial Fidelity in Vision-Language Models
Source: arXiv:2408.02231 source file (2024-08-05)
Supplement: Supplementary file 2 [file appendix_gpt_prompt.tex]

\begin{table}[!pht]\centering

\small
\begin{tabular}{l|lrlr}\toprule
\multicolumn{1}{c|}{\textbf{Input Prompt}} &\multicolumn{4}{c}{\textbf{GPT-4 Generated Coordinates}} \\
&\multicolumn{2}{c}{Object 1}  &\multicolumn{2}{c}{Object 2} \\\midrule
a cow is above a cup &cow &(5, 79) &cup &(-6, 0) \\
a broccoli is above a bus &broccoli &(15, 90) &bus &(-50, 10) \\\midrule
a knife is below an airplane &knife &(-5, 2) &airplane &(14, 86) \\
a couch is below an apple &couch &(-15, 2) &apple &(6, 90) \\\midrule
a dining table is to the left of a skateboard &dining table &(-87, 5) &skateboard &(20, -2) \\
an elephant is to the left of a hair drier &elephant &(-85, 2) &hair drier &(30, 95) \\\midrule
a vase is to the right of a fork &vase &(10, 20) &fork &(-70, 3) \\
a potted plant is to the right of a person &potted plant &(25, 30) &person &(-75, 10) \\
\bottomrule
\end{tabular}
\caption{Example Input Prompts with their respective object coordinates generated by GPT-4.}
\label{tab: gpt-prompt}

\end{table}
